# Supplementary material for: Hearing Anything Anywhere
Source: arXiv:2406.07532 source file (2024-06-11)
Supplement: Supplementary file 1 [file supmat.tex]

% % CVPR 2024 Paper Template; see https://github.com/cvpr-org/author-kit

% \documentclass[10pt,twocolumn,letterpaper]{article}

% %%%%%%%%% PAPER TYPE  - PLEASE UPDATE FOR FINAL VERSION
% % \usepackage{cvpr}              % To produce the CAMERA-READY version
% % \usepackage[review]{cvpr}      % To produce the REVIEW version
% \usepackage[pagenumbers]{cvpr} % To force page numbers, e.g. for an arXiv version

% % Import additional packages in the preamble file, before hyperref
% % \input{preamble}
% \usepackage[dvipsnames]{xcolor}

% % It is strongly recommended to use hyperref, especially for the review version.
% % hyperref with option pagebackref eases the reviewers' job.
% % Please disable hyperref *only* if you encounter grave issues, 
% % e.g. with the file validation for the camera-ready version.
% %
% % If you comment hyperref and then uncomment it, you should delete *.aux before re-running LaTeX.
% % (Or just hit 'q' on the first LaTeX run, let it finish, and you should be clear).
% \definecolor{cvprblue}{rgb}{0.21,0.49,0.74}
% \usepackage[pagebackref,breaklinks,colorlinks,citecolor=cvprblue]{hyperref}

% % Include other packages here, before hyperref.
% \usepackage{graphicx}
% \usepackage{amsmath}
% \usepackage{amssymb}
% \usepackage{booktabs}
% \usepackage{multicol}
% \usepackage{multirow}
% \usepackage{comment}
% \usepackage{float}

% \usepackage{gensymb}



% % Support for easy cross-referencing
% \usepackage[capitalize]{cleveref}
% \crefname{section}{Sec.}{Secs.}
% \Crefname{section}{Section}{Sections}

% \Crefname{table}{Table}{Tables}
% \crefname{table}{Tab.}{Tabs.}




% % New commands
% \newcommand{\name}{\textsc{DiffRIR}\xspace}


% \newcommand{\todo}[1]{\textcolor{red}{[TODO: #1]}}
% \newcommand{\sz}[1]{\textcolor{teal}{[SZ\@: #1]}}
% \definecolor{deeppurple}{rgb}{0.1, 0.0, 0.45}
% \newcommand{\mason}[1]{\textcolor{deeppurple}{[Mason\@: #1]}}
% \definecolor{deepgreen}{rgb}{0.0, 0.75, 0.96}
% \newcommand{\ryosuke}[1]{\textcolor{deepgreen}{[Ry\@: #1]}}
% \newcommand{\samuel}[1]{\textcolor{CarnationPink}{[SC\@: #1]}}
% \definecolor{nicegreen}{rgb}{0.1, 0.6, 0.2}
% \newcommand\RG[1]{\textcolor{nicegreen}{#1}}
% \newcommand{\RGnote}[1]{{\color{nicegreen}{\bf RG: }#1}}

% % Defining Colors
% \definecolor{navy}{rgb}{0.0, 0.0, 0.5}
% \definecolor{neongreen}{rgb}{0.22, 0.88, 0.08}

% \newcommand{\cameraready}[1]{{\color{neongreen}#1}}
% \newcommand{\camerareadysection}[1]{{\color{black}#1}}
% \newcommand{\myparagraph}[1]{\vspace{0pt}\paragraph{#1}}



% \makeatletter
% \renewcommand{\paragraph}{%
% \@startsection{paragraph}{4}%
% {\z@}{0.5em}{-1em}%
% {\normalfont\normalsize\bfseries}%
% }
% \makeatother

% \newcommand\rurl[1]{%
%   \href{https://#1}{\nolinkurl{#1}}%
% }



% %%%%%%%%% TITLE - PLEASE UPDATE
% \title{Hearing Anything Anywhere \\
% {\large -- Supplementary Material --}}


% %%%%%%%%% AUTHORS - PLEASE UPDATE
% % \author{Mason Long Wang\\
% % Stanford University\\
% % Institution1 address\\
% % {\tt\small ycda@stanford.edu}
% % % For a paper whose authors are all at the same institution,
% % % omit the following lines up until the closing ``}''.
% % % Additional authors and addresses can be added with ``\and'',
% % % just like the second author.
% % % To save space, use either the email address or home page, not both
% % \and
% % Second Author\\
% % Institution2\\
% % First line of institution2 address\\
% % {\tt\small secondauthor@i2.org}
% % }

% \author{
% Mason Long Wang$^1$\thanks{Equal contribution.}
% \quad
% Ryosuke Sawata$^{1,2}$$^*$
% \quad
% Samuel Clarke$^1$
% \\
% Ruohan Gao$^{1,3}$
% \quad
% Shangzhe Wu$^1$
% \quad
% Jiajun Wu$^1$ \\[0.3em]
% $^1$Stanford University
% \quad
% $^2$Sony AI
% \quad
% $^3$University of Maryland, College Park
% \\
% {\small\rurl{masonlwang.com/hearinganythinganywhere}}
% % {\tt\small ycda@stanford.edu}
% % For a paper whose authors are all at the same institution,
% % omit the following lines up until the closing ``}''.
% % Additional authors and addresses can be added with ``\and'',
% % just like the second author.
% % To save space, use either the email address or home page, not both
% }

% \begin{document}
% \maketitle

% \input{shortcut}

% {
%   \hypersetup{linkcolor=black}
%   \tableofcontents
% }
% \input{7_appendix}


% \clearpage
% %%%%%%%%% REFERENCES
% {
%     \small
%     \bibliographystyle{ieeenat_fullname}
%     \bibliography{ref}
% }


% \end{document}
